# Supplementary material for: Investigating the Benefits of Free-Form Rationales
Source: arXiv:2206.11083 source file (2022-10-25)
Supplement: Supplementary file 1 [file baseline.tex]

\section{Templates to Generate Poor-by-Construction Rationales}
\label{app:intend-incorrect}
 The ten templates we designed that aim to produce rationales that intend to be incorrect are:
 \begin{itemize}[leftmargin=*]
\vspace{-0.1in}
\itemsep-.5em
     \item if you know \emph{\{one\_of\_incorrect\_options\}}, you should know the answer to ``\emph{\{question\}}''
     \item the answer to ``\emph{\{question.lower()\}}'' is obvious based on my experience
     \item one should know \emph{\{one\_of\_incorrect\_options\}}'s relation with ``\emph{\{question.lower()\}}''
     \item the \emph{``\{question.lower()\}''}'s answer is in one of the five options
     \item answering \emph{``\{question.lower()\}''} needs some common sense reasoning
     \item it is unknown if \emph{\{one\_of\_incorrect\_options\}} can answer \emph{``\{question.lower()\}''} or not
     \item we expect \emph{\{one\_of\_incorrect\_options\}} might be able to answer \emph{``\{question.lower()\}''}
     \item answering \emph{``\{question.lower()\}''} is easy
     \item we do not know the answer to \emph{``\{question.lower()\}''}
     \item the options must contain the answer to \emph{``\{question.lower()\}''}
 \end{itemize}
 These rationales are designed to have incorrect qualities. In the ideal case, none of them should be flagged as containing background knowledge to answer a question. Therefore, we use them as a baseline to monitor the crowd-sourcing quality.
